# Supplementary material for: The Role of Linguistic Priors in Measuring Compositional Generalization of Vision-Language Models
Source: arXiv:2310.02777 source file (2023-10-04)
Supplement: Supplementary file 1 [file appendix.tex]

\begin{table*}[ht]
\caption{Standard and Hard Test Accuracies for models mentioned in Section \ref{sec:ablation}. ``EP.'' short for ``epoch''. Shown in format ``overall accuracy / hard overall accuracy / hard test accuracy'' for VG Relation and ``overall acc/hard test acc'' for the other datasets. For model names, please see explanations in Section \ref{sec:ablation}.}
\label{tab:hard-test-acc-full-appendix}
\vskip 0.15in
\begin{center}
\begin{small}
\begin{sc}
\begin{tabular}{lcccc}
\toprule
Model Name & COCO\_Order & Flickr\_Order & VG Attribution & VG Relation \\
\midrule
CLIP & 47.73 / 43.56 & 59.12 / 48.70 & 61.35 / 57.92 & 59.79 / 53.52 / 55.90\\
CLIP\_FT & 31.18 / 27.10 & 40.96 / 32.17 & 62.41 / 58.12 & 60.01 / 53.11 / 50.48\\
NegCLIP & 91.74 / 71.56 & 93.90 / 82.61 & 72.21 / 58.57 & 80.50 / 60.94 / 48.62 \\
NegCLIP (ep. 1) & 94.44 / 77.10 & 95.58 / 86.09 & 73.16 / 58.14 & 80.11 / 61.02 / 45.59\\
\midrule
CLIP\_Assist (10 trial) & 91.46 / 71.41 & 94.22 / 83.48 & 72.52 / 57.94 & 81.89 / 62.07 / 50.20 \\
CLIP\_Assist (10 trial, ep. 1) & 94.06 / 76.50 & 95.72 / 83.48 & 73.38 / 57.97 & 80.79 / 61.39 / 46.59 \\
CLIP\_Assist (30 trial) & 90.94 / 71.11 & 93.98 / 83.48 & 72.56 / 58.28 & 81.59 / 61.99 / 50.08\\
CLIP\_Assist (30 trial, ep. 1) & 93.95 / 76.05 & 95.64 / 84.35 & 73.27 / 57.61 & 80.61 / 61.28 / 46.63 \\
\midrule
CLIP\_Replace (5 trial) & 87.31 / 68.11 & 91.62 / 79.13 & 71.87 / 59.98 & 74.55 / 58.92 / 45.11\\
CLIP\_Replace (15 trial) & 83.01 / 65.72 & 88.14 / 73.04 & 70.40 /  {60.61} & 73.37 / 58.27 / 47.34 \\
CLIP\_Replace (15 trial, ep. 1) & 84.67 / 69.16 & 88.96 / 74.78 & 70.38 / 61.30 & 74.47 / 58.61 / 47.01\\
CLIP\_Replace\_2\_Diff\_POS (15 trial) & 82.93 / 62.43 & 89.16 / 76.52 & 71.77 / 60.27 & 77.05 / 59.23 / 45.83 \\
CLIP\_Replace\_2\_Diff\_POS (15 trial, ep. 1) & 86.54 / 69.31 & 90.72 / 75.65 & 72.29 / 60.52 & 75.93 / 58.76 / 44.74\\
CLIP\_Replace\_2 (15 trial)& 86.54 / 67.81 & 91.08 / 76.52 & 72.05 / 60.27 & 76.01 / 58.96 / 45.11 \\
CLIP\_Replace\_2 (15 trial, ep. 1) & 85.81 / 70.06 & 90.74 / 78.26 & 71.71 / 59.42 & 76.05 / 58.53 / 44.17\\
CLIP\_Replace\_2 (50 trial) & 82.82 / 63.92 & 88.88 / 73.91 & 71.30 / 60.41 & 75.78 / 58.87 / 45.58 \\
CLIP\_Replace\_2 (50 trial, ep. 1) & 83.01 / 66.77 & 88.56 / 73.04 & 71.42 / 59.87 & 75.67 / 58.84 / 45.65\\
\midrule
CLIP\_BERT & 44.76 / 39.37 & 49.14 / 34.78 & 62.32 / 59.58 & 62.57 / 54.56 /  {53.03} \\
CLIP\_BERT (ep. 1) & 56.30 / 45.96 & 63.30 / 50.43 & 62.46 / 59.47 & 68.01 / 55.31 / 48.45 \\
CLIP\_BERT (trial 5) & 44.51 / 34.88 & 52.26 / 40.87 & 64.71 / 59.65 & 67.27 / 56.54 / 53.43\\
CLIP\_BERT (trial 5, ep. 1) & 56.12 / 43.56 & 65.00 / 44.35 & 64.57 / 59.13 & 70.05 / 57.31 / 51.90\\
CLIP\_BERT (trial 5, 2 words) & 33.56 / 29.34 & 41.74 / 27.83 & 62.21 / 60.52 & 64.24 / 55.37 / 52.67\\
CLIP\_BERT (trial 5, 2 words, ep. 1) & 45.13 / 36.83 & 56.40 / 38.26 & 63.79 / 60.27 & 66.24 / 54.40 / 48.14\\
CLIP\_BERT (trial 15, 2 words) & 31.47 / 28.44 & 39.64 / 37.39 & 61.53 / 59.49 & 65.10 / 54.95 / 53.80\\
CLIP\_BERT (trial 15, 2 words, ep. 1) & 41.80 / 36.68 & 50.60 / 33.04 & 63.28 / 60.09 & 68.80 / 55.54 / 49.65 \\
\midrule
CLIP\_Double & 91.80 / 72.01 & 94.54 /  {86.96} &  {73.27} / 59.38 & 80.33 / 61.54 / 46.56\\
CLIP\_Double (ep. 1) &  {94.47} /  {76.95} &  {96.02} / 84.35 &  {74.10} / 59.62 & 79.61 / 61.21 / 44.29\\
\midrule
CLIP\_GPTJ & 34.10 / 29.19 & 42.88 / 28.70 & 63.65 / 59.18 & 64.62 / 55.00 / 53.41 \\
CLIP\_GPTJ (ep. 1) & 43.14 / 37.28 & 50.74 / 34.78 & 63.71 / 59.47 & 65.99 / 55.32 / 49.79 \\
CLIP\_GPTJ\_Replace & 62.52 / 50.60 & 69.82 / 56.52 & 65.02 / 57.94 & 72.09 / 58.40 / 53.19\\
CLIP\_GPTJ\_Replace (ep. 1) & 67.32 / 56.59 & 75.46 / 60.87 & 65.66 / 59.62 & 71.87 / 56.54 / 48.82\\
\midrule
CLIP\_FT (large scale) & 28.18 / 23.65 & 37.26 / 28.70 & 63.17 / 60.43 & 57.86 / 54.20 / 56.88\\
NegCLIP (large scale) & 91.27 /  {71.41} & 93.88 / 78.26 & 74.90 / 61.66 & 82.49 / 62.09 / 52.66 \\
CLIP\_Assist (large scale) &  {91.92} /  {71.41} &  {94.22} /  {81.74} & 75.89 / 61.80 &  {83.90} /  {62.78} / 51.85 \\
CLIP\_Replace (large scale) & 84.65 / 65.12 & 88.36 / 80.00 &  {76.18} /  {63.41} & 77.32 / 58.47 / 46.19\\
CLIP\_BERT (large scale) & 32.68 / 29.19 & 39.80 / 35.65 & 63.09 / 61.73 & 63.81 / 54.70 /  {58.10}\\
\bottomrule
\end{tabular}
\end{sc}
\end{small}
\end{center}
\vskip -0.1in
\end{table*}
